# Supplementary material for: Understanding new tasks through the lens of training data via exponential tilting
Source: arXiv:2205.13577 source file (2023-02-21)
Supplement: Supplementary file 1 [file supp.tex]

\section{Proofs}
\begin{proof}[Proof of Lemma \ref{lemma:eqiv-rep}]

The statement \emph{1.} is immediate. To establish \emph{2.} we note that with  $\alpha_y = - \log \left(\int p_y(x) e^{ \beta_y ^\top \Phi(x)} dx \right)$ for $y = 0$ and $1$ we have $\int p_y(x) e^{\alpha_y +\beta_y ^\top \Phi(x)}dx = 1. $ This means 
\[
\begin{aligned}
1 &= \int q_X(x)dx \\
& = \int \left(p_0(x) e^{a_0 +\beta_0 ^\top \Phi(x)}   +  p_1(x) e^{a_1 +\beta_1 ^\top \Phi(x)} \right) dx\\
& = e^{a_0 - \alpha_0} + e^{a_1 - \alpha_1}\,.
\end{aligned}\]
Letting $\pi_Q = e^{a_1 - \alpha_1}$ we have \emph{2}. 
\end{proof}

\begin{proof}[Proof of Lemma \ref{lemma:uniqueness}]
Define \[
F(\alpha_0, \alpha_1, \beta_0, \beta_1) \triangleq p_0(x) e^{\alpha_0 +\beta_0 ^\top \Phi(x)}   +  p_1(x) e^{\alpha_1 +\beta_1 ^\top \Phi(x)}\,.
\]

   For any two solutions $(a_0, a_1, b_0, b_1)$ and $(\alpha_0, \alpha_1, \beta_0, \beta_1)$ we note that $F(a_0, a_1, b_0, b_1) - F(\alpha_0, \alpha_1, \beta_0, \beta_1) = 0$ implies 
    \[
    \begin{aligned}
    p_1(x) e^{a_1 + b_1^\top \Phi(x)} + p_0(x) e^{a_0 + b_0^\top \Phi(x)} = p_1(x) e^{\alpha_1 + \beta_1^\top \Phi(x)} + p_0(x) e^{\alpha_0 + \beta_0^\top \Phi(x)}
    \end{aligned}
    \] or
    \[
    \frac{p_1(x)}{p_0(x)} = \frac{e^{\alpha_0 + \beta_0^\top \Phi(x)} - e^{a_0 + b_0^\top \Phi(x)}}{e^{a_1 + b_1^\top \Phi(x)} - e^{\alpha_1 + \beta_1^\top \Phi(x)}}
    \] which implies 
    \[
    \frac{p_1(x)}{p_0(x)} e^{u_0 + u^\top \Phi(x)} = \frac{e^{v_0 + v^\top \Phi(x)} - 1}{e^{w_0 + w^\top \Phi(x)} - 1}
    \] for $u_0 = \alpha_1 - a_0$, $u = \beta_1 - b_0$, $v_0 = \alpha_0 - a_0$, $v = \beta_0 - b_0$, $w_0 = a_1 - \alpha_1$ and $w = b_1 - \beta_1$. Since $\frac{p_1(x)}{p_0(x)} e^{u_0 + u^\top \Phi(x)} > 0$ we have
    \[
    \big(v_0 + v^\top \Phi(x)\big)\big(w_0 + w^\top \Phi(x)\big) > 0 \ \text{for any }x.
    \]
   If the range of $\Phi(x)$ is unbounded then $v \parallel w$ in a way that $v = \alpha w$ for $\alpha > 0$, which also implies $v_0 = \alpha w_0$.  From the Assumption \ref{assmp:non-linear} we conclude $v = w = 0$ or $\beta_0 = b_0$ and $\beta_1 = b_1$. Furthermore, we conclude $\alpha_0 = a_0$ and $\alpha_1 = a_1$.

   If the assumption \ref{assmp:non-linear} is not true then there exists a $\theta_0,  \delta_0\in \reals$, $\alpha>0$ and $\theta,  \delta \in\reals^d$ such that for any $x$ we have  \[p_1(x) e^{\theta_0 + \theta^\top \Phi(x)}\left(e^{\delta_0 + \delta^\top \Phi(x)} - 1\right) = p_0(x) \left(e^{\alpha\delta_0 + \alpha\delta^\top \Phi(x)} - 1\right)\,. \] If $\delta \neq 0$ then 
   \[
   p_1(x) e^{(\theta_0 + \delta_0) + (\theta + \delta)^\top \Phi(x)} + p_0(x) = p_1(x)e^{\theta_0 + \theta^\top \Phi(x)} + p_0(x)e^{\alpha \delta_0 + \alpha \delta^\top \Phi(x)}
   \] which gives non-unique values for the parameters. If $\delta = 0$ then \[
   \frac{p_1(x)}{p_0(x)} e^{\theta_0 + \theta^\top \Phi(x)} = \frac{e^{\alpha \delta_0}-1}{e^{\delta_0} - 1} > 0 \text{  or  } {p_1(x)} e^{\theta_0' + \theta^\top \Phi(x)} = p_0(x)
   \] which implies replacing $p_1(x) \gets p_0(x)e^{-\theta_0' - \theta^\top \Phi(x)}$ and $p_0(x)\gets {p_1(x)} e^{\theta_0' + \theta^\top \Phi(x)}$ we get another representation with different parameter values.
   \end{proof}

    \begin{proof}[Proof of Lemma \ref{lemma:unique-reg-fn}]
    If the solution to the equation is unique then these quantities are unique. To establish the other way we see that any two solutions $(a_0, a_1, b_0, b_1)$ and $(\alpha_0, \alpha_1, \beta_0, \beta_1)$ of the equation must satisfy \[
    \beta_0 - b_0 = \alpha(b_1 - \beta_1) \text{ and }\alpha_0 - a_0 = \alpha(a_1 - \alpha_1)
    \] for some $\alpha>0.$ If $a_1 - a_0 = \alpha_1 - \alpha_0$ and $b_1 - b_0 = \beta_1 - \beta_0$ we shall establish that $(a_0, a_1, b_0, b_1)$ and $(\alpha_0, \alpha_1, \beta_0, \beta_1)$ are same. We only establish it for $\beta_0 = b_0$ and $\beta_1 = b_1$, and the other proofs follow similarly. Replacing $b_1 \gets b_0 + \beta_1 - \beta_0$ in $\beta_0 - b_0 = \alpha(b_1 - \beta_1)$ we see that \[
    \beta_0 - b_0 = \alpha (b_0 - \beta_0) \text{ or } (1+\alpha) (\beta_0 - b_0) = 0.
    \] This implies $\beta_0 = b_0 $ and $\beta_1 = b_1$ since $\alpha> 0.$
    \end{proof}
    
\begin{theorem}[Theorem \ref{th:multi-class-exponential}]
Suppose $p_j(x), ~ q_j(x); ~ j = 1, 2, \dots, K$ are exponential family distributions with statistic $x$ and the following are satisfied. 
\begin{enumerate}
    \item $\text{span}  \Big\{ \log\big(\frac{q_j(x)}{p_j(x)}\big); ~ j = 1, \dots, K  \Big\} \subseteq \text{span} \big\{T(x), 1\big\}$.
    \item There does not exist a pair $(j, k)$, a vector $u \in \reals^{|T(x)|}$, and a scalar $v\in \reals$ such that $\frac{p_j(x)}{p_k(x)} = e^{u^\top T(x) + v}$. 
\end{enumerate} Then there exists a unique solution to the equation 
\begin{equation}
\label{eq:target-marginal-multi}
    \sum_{j = 1}^K p_j(x) \alpha_j e^{\beta_j^\top T(x) 
    } = q_X(x)\,,
\end{equation} such that $\alpha_j \ge 0$. The conditions are also necessary for existence of unique solution. 
\end{theorem}

   \begin{proof}[Proof of Theorem \ref{th:multi-class-exponential}] We will show that if the equation \eqref{eq:target-marginal-multi} has two solutions $\{\alpha_j, \beta_j\}_{j = 1}^K$ and $\{a_j, b_j\}_{j = 1}^K$ then either $a_j = \alpha_j = 0$ or $a_j = \alpha_j, ~ b_j = \beta_j $ for all $j$.  For the two solutions we have 
   \[
   \sum_{j = 1}^K p_j(x) \alpha_j e^{\beta_j^\top T(x) 
    } = \sum_{j = 1}^K p_j(x) a_j e^{b_j^\top T(x)  }
   \] Since $p_j(x) = \gamma_j e^{\delta_j^\top x}$ for some $\{\gamma_j, \delta_j\}_{j = 1}^K$ we have 

  \begin{equation}
      \sum_{j = 1}^K  \alpha_j \gamma_j e^{\beta_j^\top T(x) + \delta_j^\top x
    } = \sum_{j = 1}^K a_j \gamma_j e^{b_j^\top T(x) + \delta_j^\top x
    }
    \label{eq:non-id}
  \end{equation} 

   We require the following lemma. 
   \begin{lemma}
   \label{lemma:linear-indep}
   Let $b_1, \dots, b_T\in \reals^d$ be pairwise distinct vectors. Then $\big\{e^{x^\top b_j}\big\}_{j = 1}^T$ are linearly independent.
   \end{lemma}
   
   The condition 2. ensures that for any $j \neq k$ as a function of $x$ we have $\beta_j^\top T(x) + \delta_j^\top x \neq b_k^\top T(x) + \delta_k^\top x$,  $\beta_k^\top T(x) + \delta_k^\top x \neq b_j^\top T(x) + \delta_j^\top x$ and $b_j ^\top T(x) + \delta_j ^\top x \neq b_k^\top T(x) + \delta_k^\top x$.
   Because if either of them is not true then for some $j \neq k$ we have $(\delta_j - \delta_k)^\top x = u^\top T(x)$ for some $u$
   and this implies
   \[
   \begin{aligned}
    \log \big(\frac{p_j(x)}{p_k(x)}\big) &= (\delta_j - \delta_k)^\top x +  \log\big(\frac{\gamma_j}{\gamma_k}\big)\\
    & =u^\top T(x) + \log\big(\frac{\gamma_j}{\gamma_k}\big)\,.
   \end{aligned}
   \] This is a direct contradiction to Condition 2 in Theorem \ref{th:multi-class-exponential}. Recalling that for a full row-rank matrix $\bA$ the transformation is $T(x) = \bA x$, the condition 2. implies that for any $j \neq k$ we have $\bA^\top \beta_j + \delta_j \neq \bA^\top b_k + \delta_k$, $\bA^\top b_j + \delta_j \neq \bA^\top \beta_k + \delta_k$ and $\bA^\top b_j + \delta_j \neq \bA^\top b_k + \delta_k$. 
   
   Using the transformation $T(x) = \bA x$ the Equation \eqref{eq:non-id} can rewritten as
   \begin{equation}
       \begin{aligned}
        0 & = \sum_{j= 1}^k \alpha_j \gamma_j e^{ (\bA^\top \beta_j + \delta_j)^\top  x} - \sum_{j= 1}^k a_j \gamma_j e^{ (\bA^\top b_j + \delta_j)^\top  x}\\
        & = \sum_{j: \beta_j = b_j} \gamma_j (\alpha_j - a_j) e^{(\bA^\top b_j + \delta_j)^\top  x} + \sum_{j: \beta_j \neq b_j} \gamma_j \alpha_j e^{(\bA^\top \beta_j + \delta_j)^\top  x}\\
        & ~~~~ - \sum_{j: \beta_j \neq b_j} \gamma_j a_j e^{(\bA^\top b_j + \delta_j)^\top  x}\,.
       \end{aligned}
   \end{equation} Denoting $I \triangleq \{j: \beta_j = b_j\}$ we see that the set \[
   \{\bA^\top b_j + \delta_j\}_{j \in I} \cup \{ \bA^\top b_j +\delta_j \}_{j \in I^\complement} \cup \{ \bA^\top \beta_j +\delta_j \}_{j \in I^\complement}
   \]
   is a set of distinct vectors. 
    We now use the lemma  \ref{lemma:linear-indep} to conclude that $\gamma_j (\alpha_j- a_j) = 0$ for $j \in I$ and $\gamma_j \alpha_j = \gamma_j a_j = 0$ for $j \in I^\complement$. Since $\gamma_j \neq 0$, we conclude that \[
    \begin{cases}
    \alpha_j = a_j & \text{if} ~~ \beta_j = b_j,\\
    \alpha_j = a_j = 0 & \text{if} ~~ \beta_j \neq b_j. 
    \end{cases}
    \]  If $\beta_j \neq b_j$ for some class $j$ we have $a_j = \alpha_j = 0$, which implies the index $j$ can be eliminated from the left hand sum in equation \eqref{eq:target-marginal-multi}. This implies unique solution for the equation \eqref{eq:target-marginal-multi}.
    
   \begin{lemma}
   \label{lemma:linear-indep}
   Let $b_1, \dots, b_T\in \reals^d$ be pairwise distinct vectors. Then $\big\{e^{x^\top b_j}\big\}_{j = 1}^T$ are linearly independent.
   \end{lemma}

   \end{proof}
   
   \begin{proof}[Proof of Lemma \ref{lemma:linear-indep}] We shall prove that the only solution to the equation 
   \begin{equation}
       \label{eq:li}
       \sum_{j = 1}^T \alpha_j e^{x^\top b_j} = 0
   \end{equation} is $\alpha_1 = \dots = \alpha_T = 0$. 
   Without loss of generality we assume $\|b_T\|_2 =  \max_{j = 1,\dots, T} \|b_j\|_2$. Restricting to $x = a \frac{b_T}{\|b_T\|_2}, ~ a \in \reals$ we see that the equation \ref{eq:li} can be modified as the following. 
   \[
   \begin{aligned}
    & \sum_{j = 1}^T \alpha_j e^{u\frac{b_T^\top b_j}{\|b_T\|_2}} = 0\,,\\
   \text{or,} ~ & \sum_{j = 1}^T \alpha_j e^{u\Big(\frac{b_T^\top b_j}{\|b_T\|_2} -\|b_T\|_2 \Big)} = 0\,.
   \end{aligned}
   \] Fix $j \neq T$. If $\frac{b_T^\top b_j}{\|b_T\|_2} < \|b_j\|_2$ then $ \frac{b_T^\top b_j}{\|b_T\|_2} < \|b_j\|_2 \le \|b_T\|_2$. If $\frac{b_T^\top b_j}{\|b_T\|_2} = \|b_j\|_2$ then $b_j = \rho b_T$ for some $-1 \le \rho <1$ ($-1 \le \rho <1$ holds because $b_j \neq b_T$ and $\|b_j\|\le \|b_T\| $) which again implies $\frac{b_T^\top b_j}{\|b_T\|_2} = \rho \|b_T\|_2  < \|b_T\|_2$.
%   \[
%   \frac{b_T^\top b_j}{\|b_T\|_2} < \|b_j\|_2 \le \|b_T\|_2, ~~ \text{for any} ~ j \neq T\,,
%   \]
   
 Since $\frac{b_T^\top b_j}{\|b_T\|_2} - \|b_T\|_2 < 0$ for any $j \neq T$  letting $u \to \infty$ we get $\alpha_T = 0$. This also implies 
   \begin{equation}
       \sum_{j = 1}^{T-1} \alpha_j e^{x^\top b_j} = 0\,.
   \end{equation} We use iterative argument to conclude the lemma. 
   \end{proof}
