# Supplementary material for: Understanding new tasks through the lens of training data via exponential tilting
Source: arXiv:2205.13577 source file (2023-02-21)
Supplement: Supplementary file 4 [file SM-macros.tex]

\newcommand{\klloss}{\mathfrak{L}}
\def\heta{\widehat{\eta}}
\def\hf{{\hat f}}
\def\hP{\widehat{P}}
\def\hp{\widehat{p}}
\def\hQ{\widehat{Q}}
\def\hq{\widehat{q}}
\def\htheta{\widehat{\theta}}
\def\sf{{f^\star}}
\def\tf{{\tilde f}}
\def\htheta{{\hat \theta}}
\def\stheta{{\theta^\star}}
\def\hL{\hat L}
\def\sL{{L^\star}}
\renewcommand{\Vec}{\operatorname{vec}}
\newcommand{\breeds}{\textsc{Breeds}}
\newcommand{\waterbirds}{\textsc{Waterbirds}}
\newcommand{\strongconvexity}{\mu}
\newcommand{\nsource}{{n_P}}
\newcommand{\ntarget}{{n_Q}}
\newcommand{\weight}{\omega}
\newcommand{\coef}{\xi}
\newcommand{\scoef}{\coef^\star}
\newcommand{\hcoef}{{\hat \coef}}
